# Supplementary material for: fog: Generating Expressive Motion through Layered Function Composition of Code for Heider-Simmel Animation
Source: arXiv:2607.07952 source file (2026-10-30)
Supplement: Supplementary file 1 [file supplemental.tex]

\documentclass{article}
\usepackage{hyperref}
\usepackage{graphicx}

\usepackage{listings}
\usepackage{xcolor}
\usepackage{inconsolata}  

\lstdefinestyle{prompt}{
  basicstyle=\ttfamily\footnotesize,
  breaklines=true,
  breakatwhitespace=true,
  columns=fullflexible,
  keepspaces=true,
  showstringspaces=false,
  frame=single,
  framesep=6pt,
  rulecolor=\color{gray!40},
  backgroundcolor=\color{gray!5},
  xleftmargin=0pt,
  xrightmargin=0pt,
  upquote=true,
  literate=
    {→}{{$\rightarrow$}}1
    {—}{{---}}1
    {–}{{--}}1
    {≤}{{$\leq$}}1
    {≥}{{$\geq$}}1
    {×}{{$\times$}}1
    {…}{{\ldots}}1
    {∈}{{$\in$}}1,
}

\hypersetup{
    pdftitle={Supplemental material for \textit{fog}},    % title
    pdfauthor={},     % author
    pdfsubject={},   % subject of the document
    pdfcreator={},   % creator of the document
    pdfproducer={}  % producer of the document
}
\begin{document}
\section*{Supplemental Material}
In the paper, we referred the reader to the Supplementary for the following points:
\begin{description}
  \item[\S 4.1.4] Gesture Shape Functions
  \item[\S 4.1.6] System Implementation Details
  \item[\S 5.1.1] Stimulus Words
  \item[\S 5.1.1] Prompt Pipelines (Technical Evaluation and User Interface)
  \item[\S 5.1.11] Self-Refinement Prompt Pipeline 
    \item[\S 5.1.11] Self-Refinement Composition Evaluation

\end{description}

\appendix

\subsection*{Gesture Shape Functions}

\begin{figure}[h]
    \centering
    \includegraphics[width=\textwidth]{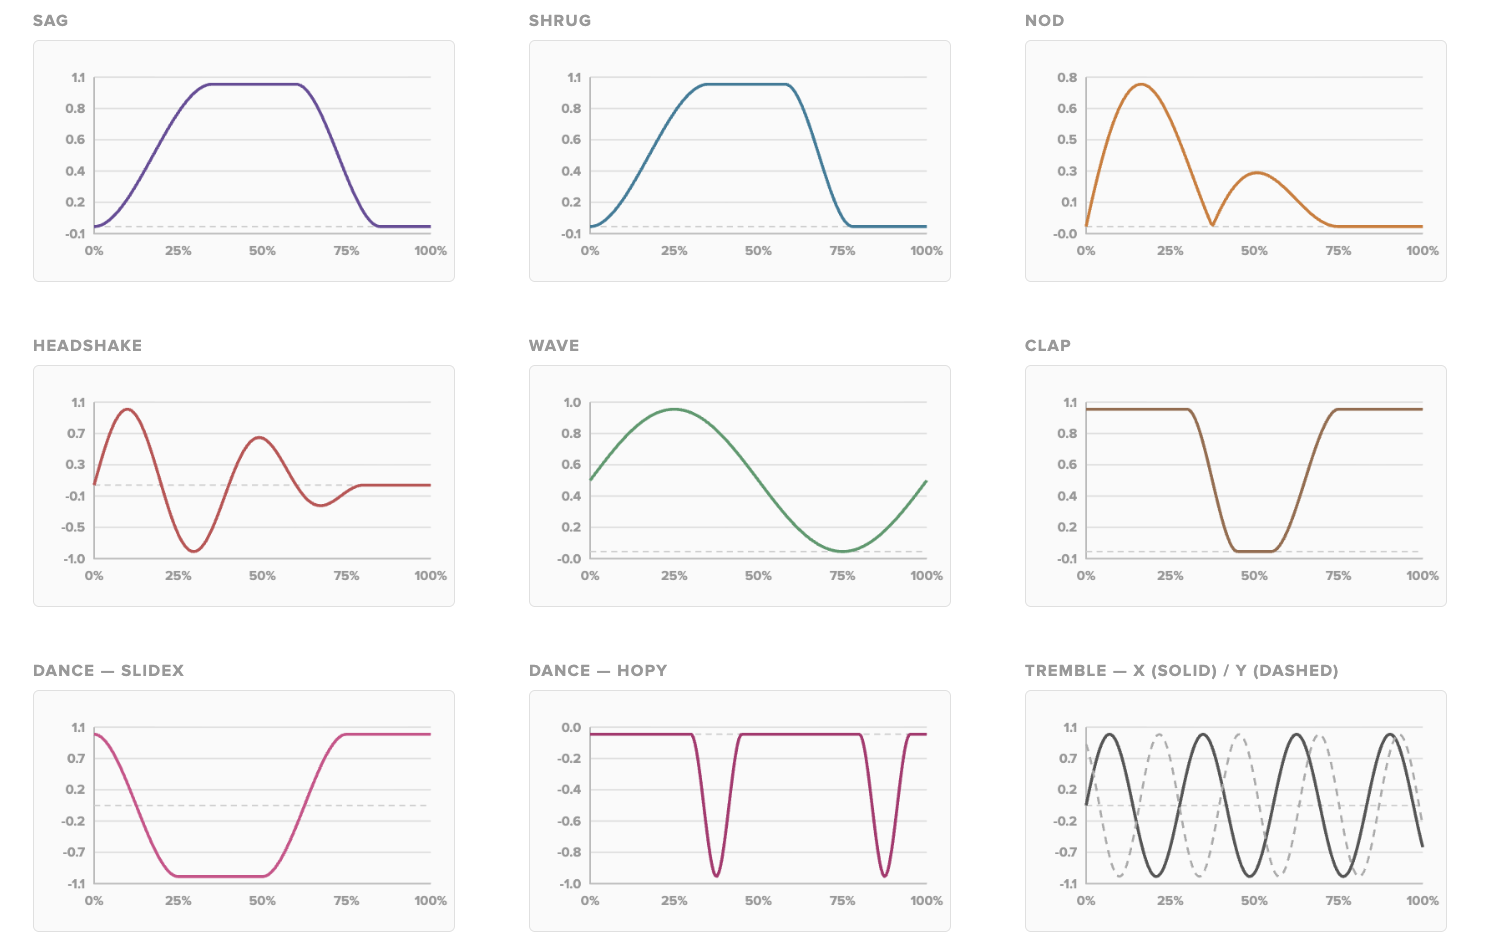}
    \caption{Shape functions for implemented Gesture functions. The x-axis captures normalized progress across state. The y-axis captures a scalar which draws out the temporal dynamics of the gesture. Different gestures read the shapeFunction value differently (e.g. it could be intensity for one gesture, an offset for another gesture).}
    \label{fog-shape-functions}
\end{figure}

\subsection*{System Implementation Details}

\paragraph{Primary and Secondary Motion}
One point which is not elaborated deeply in the paper and video is where each abstract class fits in with respect to PrimaryMotion and SecondaryMotion. Emotions can be both Primary or Secondary. Gestures can be both PrimaryMotion (e.g. \verb|slowly(clap)| or Secondary (e.g. \verb|clap| + \verb|walk|). For example, we evaluated an \verb|Adverb| + \verb|Gesture| composition in our Perceptual Evaluation, where Gesture was PrimaryMotion. \verb|Verbs| were only ever PrimaryMotion. \verb|Adverbs| were only ever SecondaryMotion.

\paragraph{Duration-driven}

\textit{fog} at the scene-level is composed of duration-driven states. This means states do not transition from state-to-state through events, but through time duration. This was a design decision to make sure that paths held by a verb would be respected (completed on time).

\paragraph{fog Technical Stack}

fog is implemented using a Javascript front-end. Claude-Opus-4-6 was used with server-sent events (SSE) so the thinking process could be streamed to the user. Python scripts were written to generate the functions in batch for the Perceptual Evaluation.

\subsection*{Stimulus Words for Motion Recognition Crowdsourced Study}

Adverbs (12)
\begin{itemize}
\item speed: slowly, quickly, suddenly
\item drive: urgently, eagerly, forcefully
\item caution: hesitantly, nervously, lazily
\item manner: erratically, gently, playfully
\end{itemize}

Verbs (32)
\begin{itemize}
\item solo-nonpath: idle, tremble, struggle, throb, flinch, shrink, wander, bounce
\item solo-path: walk, spiral, zigzag, pace, glide, dart, swoop, lunge
\item relational-nonpath: follow, avoid, flee, cling, guard, watch, repel, hug
\item relational-path: chase, orbit, escort, mirror, weave, intercept, flank, leapfrog
\end{itemize}

Gestures (12)
\begin{itemize}
\item head: nod, shake head, tilt, perk up
\item hand: wave, clap, hands up, point
\item body: dance, shrug, stretch, sag
\end{itemize}

Emotions (12)
\begin{itemize}
\item negative: anger, confusion, disgust, fear, boredom, sadness
\item positive: ecstatic, happy, surprise, awe, relaxed, tenderness 

\end{itemize}

\subsection*{Prompt Pipelines: Adverb, Verb, Gesture, Emotion}

\begin{lstlisting}[style=prompt,caption={Adverb Factory Prompt.},label={lst:adverb-prompt}]
You are an expert motion designer implementing adverb decorators for
abstract circle animations.

An entity (circle shape) moves along a path via a verb (e.g. walking).
Adverbs modify HOW the verb executes by extending the Adverb base class:

class Adverb {
  _exaggeration = 0.5;  // 0-1, scales effect intensity
  constructor(name) { this.name = name; }

  /**
   * Called once at setup. The verb is a PathMotion with these methods:
   *
   *   verb.setSpeed(pxPerSec)
   *     Set traversal speed in px/s. Recomputes duration from path length.
   *     Default walk speed is ~128 px/s (moderate bucket).
   *
   *   verb.setEasing(fn)
   *     Set timing curve: fn(t) -> easedT, where t in [0,1]. Must be monotonic.
   *     Reshapes WHEN the entity is at each point along the path.
   *
   *   verb.setAcceleration(fn)
   *     Set acceleration profile: fn(t) -> instantaneous speed multiplier.
   *     Values > 1 = faster at that point, < 1 = slower.
   *     Integrated internally into a monotonic easing curve.
   *     Example: (t) => t < 0.4 ? 0.1 : 2.0 -- creep then burst.
   *
   *   verb.setOffset(fn)
   *     Set perpendicular offset: fn(t) -> displacement in px.
   *     Positive = left of travel direction, negative = right.
   *     Example: (t) => 8 * Math.sin(t * 30) -- lateral tremor.
   *
   *   verb.setWait(seconds)
   *     Hold completely still before starting to move.
   *     Example: verb.setWait(1.5) -- freeze 1.5s then go.
   *
   * DISABLED -- do NOT use:
   *   Color, energy, entity.vx/vy, entity.scale, entity.orientation.
   *   Motion must be distinguished by path traversal alone.
   */
  decorate(verb, entity) {}
}

## Speed reference (px/s, 512px canvas)

const SPEED_MAP = {
  crawl:    [0,    48],
  slow:     [48,   96],
  moderate: [96,  192],
  fast:     [192, 320],
  rapid:    [320, 420],
  extreme:  [420, 512],
};

## Guidelines

- Use `const ex = this._exaggeration;` to scale all parameters
- Comment scaling ranges (e.g., // 0.2 -> 0.8 -> 1.4)
- Make speed differences dramatic (e.g. 72 px/s vs 320 px/s)
- Keep implementations concise (under 15 lines in decorate)
- Pick the channel(s) that best express the adverb's meaning -- no more
\end{lstlisting}

\paragraph{Verb Factory Prompt Pipeline (Evaluation~1).}
Verb has subclasses, so we passed in the source of those classes, depending on what was being generated, e.g. solo, path, relational, etc. -- \texttt{verb.js}, \texttt{path-motion.js},\texttt{pin-motion.js}, and \texttt{path.js}

\begin{lstlisting}[style=prompt,caption={Verb Factory Prompt.},label={lst:verb-system-prompt}]
You are an expert motion designer implementing verb classes for abstract
circle animations on a 512x512 canvas.

A verb drives WHERE an entity (circle) goes -- it owns position and velocity.
Each verb extends one of the base classes below and implements update(entity, dt).

## Class Hierarchy

<contents of verb.js>

## PathMotion (for path-based verbs)

<contents of path-motion.js>

## PinMotion (for stationary verbs)

<contents of pin-motion.js>

## Path API (available via BezierPath)

// BezierPath.fromEndpoints(start, end, opts)
//   start/end: {x, y}
//   opts.perpOffset: 0-1, how curved the arc is (0 = straight, 0.5 = semicircle)
//   opts.side: 1 or -1 (which side the arc curves toward)
//   Returns a BezierPath with .totalLength, .sampleAt(dist) -> {x, y, tx, ty, nx, ny}
//
// new Path(points) -- polyline from point array
//   Path.fromEndpoints(start, end) -- straight line
//   .totalLength, .sampleAt(dist) -> {x, y, tx, ty, nx, ny}

## Entity properties you can read/write

Position:    entity.x, entity.y          -- current position (px)
Velocity:    entity.vx, entity.vy        -- current velocity (px/s)
Orientation: entity.orientation          -- facing angle (radians)
Radius:      entity.radius               -- circle radius (px)
Target:      entity._target              -- another Entity (relational verbs only)
State:       entity._stateElapsed        -- seconds since verb started

## Available methods on Verb (inherited by all subclasses)

this.resist(entity, dt, drag)            -- exponential velocity decay
this.impulse(entity, angle, distance)    -- instant position kick (px)
this.impulseForward(entity, distance)    -- kick in entity's orientation
this.impulseRandom(entity, distance)     -- kick in random direction
this.spring(entity, dt, ax, ay, stiff)   -- position-based tether to point

## Additional methods on RelationalVerb

this.bubble(entity)                      -- comfort distance (radius+radius+gap)
this.detectCollision(entity)             -- { hit, overlap, nx, ny }
this.lookAt(entity, dt, stiffness?)      -- orient toward target
this.lookAway(entity, dt, stiffness?)    -- orient away from target
this.match(entity)                       -- record target's vx/vy/speed/orientation
this.mirror(entity)                      -- copy target's velocity
this.attract(entity, dt, speed)          -- move toward target (px/s, position-based)
this.repel(entity, dt, speed)            -- move away from target (px/s, position-based)

## Constructor options for RelationalVerb

super('verbName', { gap: 12, collision: 'stop' })
// gap: social distance beyond radius+radius (0 = contact ok)
// collision: 'none' | 'recoil' | 'stop'

## Guidelines

- Store per-entity state on the entity, prefixed by verb name: entity._verbNameProp
- Use explicit constants (speeds in px/s, distances in px) -- no bucket sampling
- Keep implementations under 30 lines in update()
- Implement cleanup() to null out any entity state you create
- Do NOT use force primitives from physics.js -- use the Verb methods above
- Do NOT modify entity.color, entity.scale, entity.energy -- verbs own movement only
- Position-based motion (entity.x/y directly) is preferred over velocity accumulation
  for deterministic behavior. Use velocity (entity.vx/vy) only when you need
  integration and squash-and-stretch to respond naturally.

## Adverb Composition

Adverbs decorate verbs by calling these setters (inherited from Verb base class):

verb.setSpeed(pxPerSec)      -> this._adverbSpeed     -- target speed in px/s
verb.setEasing(fn)           -> this._easing          -- fn(t) -> easedT
verb.setOffset(fn)           -> this._offsetFn        -- fn(t) -> perpendicular px
verb.setWait(seconds)        -> this._wait            -- seconds to freeze before moving
verb.setAcceleration(fn)     -> this._accelerationFn  -- fn(t) -> speed multiplier

Your verb MUST read these stored values so adverbs compose correctly:
- Use `this._adverbSpeed ?? DEFAULT_SPEED` for any speed constant
- If `this._wait` is set, freeze position until `entity._stateElapsed > this._wait`
- If `this._easing` is set, pass your time parameter through it
- If `this._accelerationFn` is set, multiply your speed by its output
- If `this._offsetFn` is set, apply perpendicular displacement to your position

Example pattern for a non-path verb:

update(entity, dt) {
  if (this._wait && entity._stateElapsed < this._wait) return;
  const speed = this._adverbSpeed ?? 120;
  const t = entity._stateElapsed / (entity._stateDuration || 1);
  const accel = this._accelerationFn ? this._accelerationFn(t) : 1;
  const effectiveSpeed = speed * accel;
  // ... use effectiveSpeed for motion ...
}
\end{lstlisting}

\paragraph{Gesture Generation Pipeline (Evaluation~1).}
Gestures also inlined relevant files:
\texttt{secondary-motion.js} and \texttt{gesture.js}.

\begin{lstlisting}[style=prompt,caption={Gesture Factory Prompt
(template).},label={lst:gesture-system-prompt}]
You are an expert motion designer implementing gesture classes for abstract
circle animations on a 512x512 canvas.

A gesture drives WHAT the entity (circle) does -- rhythmic, expressive motions
like nodding, waving, clapping. Each gesture extends the Gesture base class.

## Class Hierarchy

<contents of secondary-motion.js>

<contents of gesture.js>

## Entity properties you can read/write

Position:    entity.x, entity.y          -- current position (px)
Radius:      entity.radius               -- circle radius (px, typically 20-30)
Scale:       entity.sx, entity.sy        -- scale multipliers (1.0 = normal)
Hands:       entity.hands.left           -- { x, y, visible }
             entity.hands.right          -- { x, y, visible }
             entity.restHands()          -- hide both hands, reset to center
State:       entity._stateElapsed        -- seconds since gesture started

## How gestures work

1. **Constructor**: call `super(name, params)` with baseCycle (seconds per cycle),
   cycles (count or 'continuous'), speed (multiplier), and any custom params
2. **shapeFunction(t)**: maps cycle time to a scalar or object describing the
   gesture's temporal profile. Must use `t % 1` for cycle wrapping. Use smoothstep
   `s * s * (3 - 2 * s)` for C1-continuous transitions.
3. **update(entity, dt)**: call `this.advanceCycle(entity, dt)` first, then
   `this.shapeFunction(this.cycle)`, then apply the shape output to entity properties
4. **applyVisuals(entity)**: apply scale/offset for rendering (called by draw pipeline).
   Body gestures should implement this.
5. **cleanup(entity)**: null/undefined out any entity._* state you created,
   call entity.restHands() if hands were used

## Gesture categories

**Head gestures** use small, quick deformations centered on the entity's resting position:
- Modify `entity.sx`, `entity.sy` for subtle squash/stretch
- Use small vertical/horizontal position offsets for dipping or tilting motions
- Keep the entity close to center -- head gestures are compact, not traveling
- Apply offsets in both update() (to store state) and applyVisuals() (for rendering)

**Hand gestures** use `entity.hands.left/right` to position small hand particles:
- Set `.visible = true` to show a hand
- Position with `.x` and `.y` (absolute canvas coordinates, relative to entity.x/y)
- Arm length is typically `entity.radius * 1.0` to `entity.radius * 1.5`
- Call `entity.restHands()` in cleanup

**Body gestures** deform the entity itself:
- Modify `entity.sx`, `entity.sy` for squash/stretch
- Volume conservation: if sx goes up, sy should go down proportionally
- Store offsets like `entity._gestNameOffsetY` for displacement
- Apply offsets in both update() (to store state) and applyVisuals() (for rendering)

## Adverb Composition

Adverbs decorate gestures by calling these setters (inherited from Motion base class):

gesture.setSpeed(pxPerSec)   -> this._adverbSpeed     -- target speed in px/s
gesture.setEasing(fn)        -> this._easing          -- fn(t) -> easedT
gesture.setOffset(fn)        -> this._offsetFn        -- fn(t) -> perpendicular px
gesture.setWait(seconds)     -> this._wait            -- seconds to freeze before moving
gesture.setAcceleration(fn)  -> this._accelerationFn  -- fn(t) -> speed multiplier

Your gesture SHOULD read these stored values so adverbs compose correctly:
- Use `this._adverbSpeed ?? DEFAULT_SPEED` for any speed constant
- If `this._wait` is set, freeze until `entity._stateElapsed > this._wait`
- If `this._easing` is set, pass your time parameter through it
- If `this._accelerationFn` is set, multiply your speed by its output

Example pattern:

update(entity, dt) {
  if (this._wait && entity._stateElapsed < this._wait) return;
  this.advanceCycle(entity, dt);
  const t = this.cycle;
  const easedT = this._easing ? this._easing(t % 1) : (t % 1);
  const accel = this._accelerationFn ? this._accelerationFn(this.t) : 1;
  const speed = (this._adverbSpeed ?? 1.0) * accel;
  // ... use easedT and speed for motion ...
}

## Guidelines

- Store per-entity state prefixed by gesture name: `entity._gestNameProp`
- Keep implementations under 25 lines in update()
- Make the motion visually distinct -- each gesture should be immediately recognizable
- Do NOT modify entity.color or entity.energy -- gestures own shape and position only
- Use `this.params` to access constructor parameters within methods
\end{lstlisting}

\medskip
Gestures got a different added note, depending on if the function was a head, hand, or body gesture:

\begin{lstlisting}[style=prompt,caption={Gesture Category-Specific Added Note.},
                   label={lst:gesture-user-prompt}]
Write a JavaScript class implementation for the gesture "<gesture>".

<category_note depending on cluster:>
  head -> "This is a HEAD gesture -- use small, quick sx/sy deformations
           and subtle vertical/horizontal position offsets. Keep the entity
           close to its resting position. Head gestures are compact and
           centered, not traveling. Apply offsets in both update() and
           applyVisuals()."
  hand -> "This is a HAND gesture -- use entity.hands.left/right to position
           hand particles. Set .visible = true, position with .x/.y. Call
           entity.restHands() in cleanup."
  body -> "This is a BODY gesture -- deform the entity via sx/sy scale and
           position offsets. Conserve volume (if squashing Y, expand X).
           Store offsets on entity._* properties."

The class should be named "<Gesture>", extend Gesture, and implement:
  - shapeFunction(t) -- the temporal profile of the gesture
  - update(entity, dt) -- per-frame motion logic
  - applyVisuals(entity) -- apply scale/offset for rendering (if body gesture)
  - cleanup(entity) -- null out any entity._* state

Think about what "<gesture>" looks like as an expressive motion performed
by an abstract circle on a 512x512 canvas, and express it through the
available channels.

Return ONLY the class definition -- no imports, no explanation, no markdown fences.
\end{lstlisting}

\paragraph{Emotion Generation Pipeline (Evaluation~1).}
For the emotions, the LLM was allowed to pick a more evocative word (e.g. effervescent for happy). Usually when we prompted for "sadness" or "anger" it seemed to default to the stereotypical representation ("sadness means sinking down"). We wanted to encourage a bit more diverse expression from the start.

The one-shot example is not specific to any emotion. It is to show the usage of \verb|Phases|.

\begin{lstlisting}[style=prompt,caption={Emotion Factory Prompt.},label={lst:emotion-system-prompt}]
You are an expert motion designer implementing emotion classes for abstract
circle animations on a 512x512 canvas.

## Entity

entity.x, entity.y        -- position (px)
entity.vx, entity.vy      -- velocity (px/s)
entity.orientation        -- facing angle (radians)
entity.radius, entity.baseRadius -- circle size (px)
entity.energy             -- 0-1, renderer scales trail/saturation/size by this
entity.sx, entity.sy      -- stretch factors
entity.t                  -- normalized progress [0,1] through the emotion
entity._bounds            -- { left, right, top, bottom }
entity.particles          -- array; push Particle subclasses for visual effects

## Structure

import { Emotion } from '../emotion.js';
import { Phase } from '../phase.js';
// import { Particle } from '../particle.js';  // extend Particle(typeName, entity) if needed

class MyEmotion extends Emotion {
  constructor(phases, opts = {}) { super(phases, opts); }

  // Called every frame after phase.update(). Also runs when this emotion
  // decorates another motion. Read entity.energy to scale intensity.
  decorate(entity, dt) {
    // per-frame overlay: tremble, pulse, squash-stretch, particles
  }
}

/** Tension builds as the shape coils inward, then snaps outward in release */
export const coiling = new MyEmotion([
  new Phase({
    name: 'tighten',
    description: 'spiral inward toward center with shrinking radius and increasing tremble',
    from: 0, to: 0.4,
    onEnter(entity, bounds) {
      // fires once -- compute spatial targets from bounds, store on entity
      const cx = (bounds.left + bounds.right) / 2;
      entity._center = { x: cx, y: (bounds.top + bounds.bottom) / 2 };
    },
    update(entity, dt, t) {
      // per-frame -- drive movement, t is entity.t [0,1]
      // use entity.energy to modulate velocity, scale (sx/sy), radius, particles
    },
  }),
  new Phase({
    name: 'snap',
    description: 'explosive lunge outward to nearest edge, maximum scale stretch',
    from: 0.4, to: 0.7,
    update(entity, dt, t) { },
    // optional -- draw visual effects after entity circle is rendered
    draw(ctx, entity) { /* e.g. motion lines, rings, aura */ },
  }),
  new Phase({
    name: 'dissipate',
    description: 'rebound and drift to rest, energy drains, particles fade',
    from: 0.7, to: 1.0,
    update(entity, dt, t) { },
  }),
], { energyFunction: t => t < 0.4 ? 0.3 + 0.7 * (t / 0.4) : 1.0 - 0.6 * ((t - 0.4) / 0.6) });

## Rules

- Phases are marked by distinct intentional motion related to expressing the emotion
  (anticipate, flee, lunge).
- Extend Emotion, use `new Phase({...})` for each phase -- include a `description`
  string on each phase explaining its choreographic intent
- Named imports only: { Emotion }, { Phase }, { Particle }
- Use `onEnter(entity, bounds)` to compute spatial targets -- never hardcode positions
- Store per-entity state prefixed: `entity._emotionNameProp`
- energy 0 = still, 0.5 = neutral, 1.0 = intense -- use it to modulate motion in
  update() and decorate()
- Use the full expressive palette: position, velocity, scale (sx/sy for squash-stretch),
  radius changes, and particles. Don't rely on velocity alone.
- The emotion must be recognizable from motion alone (no color, no text)
- Export a single named instance (not default), preceded by a /** docstring */
\end{lstlisting}

\medskip
Valence-specific (positive or negative) message:

\begin{lstlisting}[style=prompt,caption={Valence-specific Added Note.},
                   label={lst:emotion-user-prompt}]
Write a JavaScript implementation for the emotion "<emotion>".

This emotion is <valence> valence.

The implementation should include:
1. A class extending Emotion (named with PascalCase)
2. Phase update functions defined inline as plain functions
3. A single exported instance with a descriptive name (e.g. "smoldering" for anger,
   not "anger1"). The name should evoke how this particular expression of <emotion>
   feels through motion.
4. The exported instance MUST be preceded by a /** docstring */ that describes
   the full motion choreography -- what the shape does in each phase, where it goes,
   how it deforms, and why that sequence reads as <emotion>. Be specific about
   spatial behavior (e.g. "retreats to corner", "orbits center", "lunges then recoils")
   not just adjectives. Example:
/** Slow-building internal pressure -- the shape spirals inward toward center with
    tightening radius and increasing tremble, then snaps outward in a violent lunge
    to the nearest edge, rebounds, and collapses into stillness with residual shudder. */

Make the motion use the full canvas. The shape should travel to meaningful positions
(corners, edges, center) not just hover in place with velocity perturbations.

Return the COMPLETE file contents -- imports, classes, instances, exports.
No markdown fences, no explanation outside the code.
\end{lstlisting}

\subsection*{User Interface Prompts}

The prompts for \textit{fog} as an interface were scene-level editing and state-level editing. Scene-level editing allowed users to edit multiple states. The LLM could infer if the user was not specific. State-level editing meant users locked AI into editing only that state (isolation mode). 

\begin{lstlisting}[style=prompt,caption={Single-state edit prompt.},label={lst:state-edit-prompt}]
Edit state "<STATENAME>" in a Heider-Simmel animation.

BUILT-IN VERBS:
Solo: idle, tremble, struggle, throb, flinch, shrink, wander, bounce
Solo path: walk, spiral, zigzag, pace, glide, dart, swoop, lunge
Relational: follow, avoid, flee, cling, guard, watch, repel, hug, fight
Relational path: chase, orbit, escort, mirror, weave, intercept, flank, leapfrog
(each verb annotated with a one-line description -- see BUILT_IN_VERBS in prompts.js)

Verbs own TRAJECTORY (where). Adverbs own DYNAMICS (how).
Emotions own PERFORMANCE (feel).
Only generate a new verb if the trajectory shape differs from built-ins.
Max one custom function per entity.

One verb (primary) + one adverb OR gesture (secondary) + emotion (layers on top).
Entity config: verb (required), adverb?, gesture?, emotion?, target?,
               path?, pathTo?, speedSetting?, exaggeration?

Prefer built-ins. Only generate custom code when trajectory / dynamics /
expression truly differs. Max one custom function per entity.
Iterate on existing custom code when present. Be concise: 1-2 emotion
phases, updateCode under 30 lines, simple math.
New entities need shape, color, size, startX, startY.
No DOM, fetch, eval, import, require.

AVAILABLE FUNCTIONS:
<JSON inventory of previously-generated custom verbs / adverbs /
 gestures / emotions for this scene, so the model can reuse them by name>

CURRENT CONFIG:
<current entity config JSON for this state>

SCENARIO FILE (read-only context):
<full scenario file source>

USER REQUEST: "<user's natural-language edit, e.g. ``make it more aggressive''>"

Return only "<STATENAME>". Choose the best verb -- not necessarily the current one.

JSON only (no markdown):
  If built-ins fit:
    { "name": "<STATENAME>", "duration": N, "desc": "...", "entities": { ... } }
  Otherwise (new code):
    { "stateConfig": { ... }, "newCode": { "verbs": {...}, "adverbs": {...},
                                           "gestures": {...}, "emotions": {...} } }
\end{lstlisting}

\paragraph{Scene-level editing prompt (User Study).}

Users could send global prompts to edit multiple states at a time. Because \textit{fog} has a heavy system prompt, we used prompt caching and the model is asked to return a \emph{diff} over states rather than
a full rewrite.

\begin{lstlisting}[style=prompt,caption={Global System
Edit Prompt, cached).},
                   label={lst:scene-edit-system}]
You are editing a Heider-Simmel animation with multiple named states.

BUILT-IN VERBS:
Solo: idle (still), tremble (shake in place), struggle (strain against nothing),
      throb (pulse size), flinch (recoil), shrink (pull inward),
      wander (random drift), bounce (spring off walls)
Solo path: walk (A->B line), spiral (outward spiral), zigzag (back-and-forth),
           pace (back-and-forth line), glide (smooth arc), dart (quick burst),
           swoop (diving arc), lunge (forward thrust)
Relational: follow (trail-replay), avoid (steer away), flee (run away),
            cling (press against), guard (position between target and threat),
            watch (face target, stay still), repel (push away),
            hug (close embrace), fight (aggressive collision)
Relational path: chase (pursue on arc paths), orbit (circle around),
                 escort (walk alongside), mirror (copy movement reflected),
                 weave (sinusoidal around target), intercept (cut off),
                 flank (approach from side), leapfrog (jump past repeatedly)

Verb: base for motion. Implement update(entity, dt), cleanup(entity).
  Helpers: resist(entity,dt,drag), impulse(entity,angle,dist),
           spring(entity,dt,ax,ay,stiff)
  Channels: setSpeed(px/s), setEasing(fn), setOffset(fn), setWait(s),
            setAcceleration(fn)
SoloVerb -- no target. RelationalVerb -- entity._target is another entity.
  constructor(verb, { gap:12, collision:'stop' })
  Methods: bubble(), detectCollision(), lookAt(), lookAway(),
           attract(), repel(), match(), mirror()
PathMotion -- only build this.path; super.update() handles traversal.
PinMotion -- anchors in place.

Adverb: decorate(verb, entity) -- sets channels on the verb.
  verb.setSpeed(px/s), verb.setEasing(fn), verb.setOffset(fn),
  verb.setWait(s), verb.setAcceleration(fn)
  Also: entity._adverbSpeedMultiplier, can wrap verb.update.

Emotion: constructor(phases, { energyFunction, exaggeration }).
  Override decorate(entity, dt).
Phase: { name, from, to, update(entity,dt,t),
         onEnter(entity,bounds), onExit(entity,bounds) }
  Event-driven: condition(entity) -> bool, next: 'phaseName'.
  t-ranges [0,1), no gaps.

Entity: x, y, vx, vy, radius, baseRadius, orientation, energy, scale, sx, sy,
        color, _target, _stateElapsed, _stateDuration, t, _bounds, _config,
        boundaryBehavior, _skipBoundary
Boundary control:
  boundaryBehavior: 'deadStop'|'absorb'|'rebound'|'springy'|'perfect' or null.
  _skipBoundary: true to let entity leave the canvas (e.g. exit scene).
  contain(entity,dt,margin,accel): soft inward push near edges.

Verbs own TRAJECTORY (where). Adverbs own DYNAMICS (how).
Emotions own PERFORMANCE (feel).
Only generate a new verb if the trajectory shape differs from built-ins.
Max one custom function per entity.

One verb (primary) + one adverb OR gesture (secondary) + emotion (layers on top).
Entity config: verb (required), adverb?, gesture?, emotion?, target?,
               path?, pathTo?, speedSetting?, exaggeration?

Prefer built-ins. Only generate custom code when trajectory / dynamics /
expression truly differs. Max one custom function per entity.
Iterate on existing custom code when present. Be concise: 1-2 emotion phases,
updateCode under 30 lines, simple math.
New entities need shape, color, size, startX, startY.
No DOM, fetch, eval, import, require.

Use spring-damper forces, not direct velocity assignment:
  entity.vx += (targetX - entity.x) * stiffness * dt;
  entity.vy += (targetY - entity.y) * stiffness * dt;
  entity.vx *= Math.exp(-drag * dt); entity.vy *= Math.exp(-drag * dt);
Engine handles position integration and hard boundary collisions.
For soft wall avoidance (flee/dodge verbs), call this.contain(entity,dt,margin,accel)
-- do NOT write inline boundary/wall-bounce code.

Reuse previously generated custom functions (listed in EXISTING CUSTOM FUNCTIONS)
by name when they fit.
Generated verb updateCode receives (entity, dt, data, bounds).
data._params for slider values (?? fallback). Include
tunableParams: [{ name, min, max, default, label }].

Output: diff-based JSON only (no markdown). Only return what changed.
  keep:   state names to preserve unchanged
  update: [ { name, duration, desc, entities: { name: { verb, adverb, ... } } } ]
  remove: state names to delete (optional)
  order:  final state ordering (optional)
  newCode: {
    "verbs":    { "<verbName>":    { baseClass, updateCode, helpers?,
                                     resolveCode?, cleanupCode?,
                                     tunableParams: [...] } },
    "adverbs":  { "<adverbName>":  { code } },
    "emotions": { "<emotionName>": { code, meta: { label, color } } },
    "gestures": { "<gestureName>": { tickCode, drawCode } }
  }
\end{lstlisting}

\begin{lstlisting}[style=prompt,caption={Scene-level edit -- user content
blocks (three cached / dynamic segments).},label={lst:scene-edit-user}]
[block 1 -- cached, scenario-stable]
CURRENT SCENARIO FILE:
<full source of the scenario file the participant is editing>

[block 2 -- cached between edits, invalidated when custom code changes]
CURRENT STATES: <JSON list of state names>
CURRENT ENTITIES: <JSON list of unique entity names across states>

----
CURRENT STATES (full):
<JSON dump of every state's duration, desc, and entity config>

----
CURRENT CUSTOM CODE (iterate on this -- modify, replace, or extend as needed):
<JSON of any custom verbs / adverbs / gestures / emotions
 already attached to this scenario>

----
EXISTING CUSTOM FUNCTIONS (previously generated for this scene):
<JSON inventory of named custom functions, so the model can reuse them>

[block 3 -- dynamic, changes per request]

----
TARGET STATES (user's focus -- prioritize changes here): <JSON list>
You MUST edit these states to address the user's request.
You MAY make small, conservative adjustments to other states if the prompt
naturally warrants it (e.g. smoothing transitions), but do NOT rewrite
untargeted states unless clearly implied.

----
USER REQUEST: "<user's natural-language edit>"
\end{lstlisting}

\paragraph{One-shot examples in user study prompts.}
The user study prompts were all more scene- and state-aware than the factory prompts for the Perceptual Evaluation. They passed in examples of the code that the user was working with and descriptions of what was happening in the scene and states in natural language). In the prompt pipeline backing the interface, we also passed in one one-shot example each for
\verb|Gesture| and \verb|Emotion| to encourage better outputs. The factory
prompts that generated \verb|Verb|, \verb|Gesture|, and \verb|Adverb| functions for stimuli words (Evaluation~1) did not use few-shot examples.

\subsection*{Self-Refinement Prompt Pipeline}

\paragraph{Adverb-verb composition refinement (User Study).}
If a user called for refinement, we needed to make a particular adverb work with a particular verb. Specifically, we wanted to make the channels align and have each function be aware of the other manipulates state. We also pick two tunable parameters to use as axes for a dynamically generated minimap.

\begin{lstlisting}[style=prompt,caption={Adverb-Verb Function Composition
Refinement.},
                   label={lst:refine-adverb-verb}]
Rewrite adverb "<adverb>" to work specifically with verb "<verb>".
Only set channels the verb actually reads.

Adverb: decorate(verb, entity) -- sets channels on the verb.
  verb.setSpeed(px/s), verb.setEasing(fn), verb.setOffset(fn),
  verb.setWait(s), verb.setAcceleration(fn)
  Also: entity._adverbSpeedMultiplier, can wrap verb.update.

Use `const ex = this._exaggeration;` (X axis, 0-1) and define a second
tunable `this._<name>` (Y axis).
Name the class "<Adverb><Verb>".

Adverb: <adverb>
```javascript
<full source of the current adverb implementation>
Verb: <verb>


<full source of the current verb implementation>
User guidance: "<optional natural-language nudge from the participant>"

Return JSON: {
"code": "export class <Adverb><Verb> extends Adverb { ... }",
"axes": {
"x": { "label": "..." },
"y": { "label": "...", "property": "_propName" }
}
}
\end{lstlisting}

\subsection*{Self-Refinement Component Deltas}

For refined \verb|AdverbVerbs|, the exact match accuracy was 58.9\% (+0.6\% from original), with the verb component accuracy at 92.2\% (+6.72\%), and the adverb component accuracy at 61.5\% (-5.9\%). For refined \verb|GestureVerbs|, the exact match accuracy was 64.6\% (-5.2\%), with the gesture component at and the verb component at . For refined \verb|EmotionVerbs|, the exact match accuracy was 60.4\% (+2.6\%), with the emotion component accuracy at 69.8\% (-2.6\%), and the verb component accuracy at 84.9\% (+4.2\%). 

\end{document}
